# Supplementary material for: Quantifying and Localizing Usable Information Leakage from Neural Network Gradients
Source: arXiv:2105.13929 source file (2022-07-25)
Supplement: Supplementary file 1 [file appendix.tex]

\section{Appendix}
\label{sec:appendix}

\subsection{Existing attacks}
\label{sec:attacks_sum}
\begin{table*}[htbp]
  \centering
  \caption{Existing attacks. \moh{Maybe better to have two sub-parts, one for PIAs and one for DRAs} \vin{there is only one PIA :D}}
    \begin{tabular}{|p{2.415em}|r|p{2.75em}|p{16em}|p{12em}|p{17em}|}
    \hline
    Ref.  & \multicolumn{1}{p{2.5em}|}{Year} & Attack\newline{}type & Attack models & Scenarios & Results/Performance \bigstrut\\
    \hline
    \cite{melis2019exploiting} & 2019  & PIA   & Tested logistic regression, gradient boosting, and random forests; random forests with 50 trees performed the best & One client uses global model's multiple snapshots, to infer others' properties & 2-24 users, batch 32-1000 depends on datasets (image or texts), 0.6-0.9 precision \bigstrut\\
    \hline
    \cite{wang2019beyond} & 2019  & DRA   & A framework incorporating GAN with a multi-task discriminator & Attack on shared gradients (actively) using gobal model's multiple snapshots & 10-40 users, up to 64x64 images  \bigstrut\\
    \hline
    \cite{zhu2019deep} & 2019  & DRA   & Optimization method that minimizes the dummy gradients distance to recover & Attack on shared gradients directly from others & 1-8 batch size, 32x32 (100 classes) and 64x64 images \bigstrut\\
    \hline
    \cite{zhu2020r} & 2020  & DRA   & A closed-form recursive procedure; a Rank Analysis method to estimate the privacy risk & Attack on shared gradients directly from others & 1-5 batch size, 32x32 images with 100 classes \bigstrut\\
    \hline
    \cite{geiping2020inverting} & 2020  & DRA   & By exploiting a cosine similarity loss along with optimization methods from adversarial attacks & Attack on shared gradients directly from others & 5 most recognizable images from a batch of 100, 32x32 images with 100 classes (up to ImageNet); analytcally reconstruct from only fully connected layers \bigstrut\\
    \hline
    \cite{yin2021see} & 2021  & DRA   & An optimization method; a group consistency regularization framework to enhance reconstructed data & Attack on shared gradients directly from others & 8-48 batch size, up to 224x224 images with 1000 classes \bigstrut\\
    \hline
    \moh{\cite{he2019model}}& & DRA &  \vin{this one seems to use internal representation from inference to conduct the attack. Not sure this is our aiming attack} \moh{Yeah. Maybe we can have them here as attacks that are not applicable. So, this table can serve as a table that shows what kind of DRA are actually possible in collaborative SGD. } & \bigstrut\\
    \hline
    \moh{\cite{yang2019neural,zhang2020secret}}&&DRA &\vin{these two seem to be standard ML not collaborative, aka no gradient sharing.}& \bigstrut\\
    \hline
    \end{tabular}%
  \label{tab:addlabel}%
\end{table*}%

\subsection{Federated learning setting}
We consider a user who participates in a {\em collaborative} training task for a number of {\em iterations} $K$. The user owns a private dataset including $M$ samples $D = \{(X^m,Y^m)\}_{m=1}^{M}$. The dataset $D$ has one {\em latent attribute} $p$ which is the same for all samples $X^m$.
At each round $k \in \{1,\dots,K\}$, the user trains the received model $\mathcal{F}^{k-1}$ for a number of {\em epochs} $E$. At each epoch $e \in \{1, \dots, E\}$, the user optimizes the model $\mathcal{F}^{k-1}_{e} \leftarrow \mathcal{F}^{k-1}_{e-1}$ via SGD method. At the end of each iteration $k$, the user sends to the server, the difference between the received model $\mathcal{F}^{k-1}$ and latest updated model $F^{k} \leftarrow \mathcal{F}^{k-1}_{E}$ which we call it $G = \mathcal{F}^{k} - \mathcal{F}^{k-1}$. When there is only one epoch,\ie $E=1$, and this epoch uses only one SGD round on the whole dataset $D$, then $G$ is basically the average {\em gradient} of $D$ with respect to $\mathcal{F}^{k-1}$. When $E>1$, then $G$ is the aggregated gradients of multiple SGD optimization rounds. 

\moh{@Vincent: How do you perform each epoch? is it one round of SGD with a batch size equal to the size of the uesr's dataset? or is it multiple round of SGD with a small batch size?} \vin{it's mini batch SGD}
